# Supplementary material for: Assessing the correctness of pressure correction to solvation theories in the study of electron transfer reactions
Source: arXiv:2102.11616 source file (2021-03-10)
Supplement: Supplementary file 1 [file SI.pdf]

# Supporting information: Assessing the correctness of pressure correction to solvation theories in the study of electron transfer reactions

Tzu-Yao Hsu[1] and Guillaume Jeanmairet[1,2]

[1] *Sorbonne Université, CNRS, Physico-Chimie des Électrolytes et Nanosystèmes Interfaciaux, PHENIX, F-75005 Paris, France*

[2] *Réseau sur le Stockage Électrochimique de l'Énergie (RS2E), FR CNRS 3459, 80039 Amiens Cedex, France*

# I. THE BREAKDOWN OF FUNCTIONAL DIFFERENCE

In the main paper, we computed the change in the reorganization free energy upon adding the WDA correction (equation 15 of the main paper) for an ionic oxydation state $\alpha$. Recalling that the external potential is the sum of a Lennard-Jones (LJ) and an electrostatic (elec) contribution and using equation 1 and 13 of the main paper this quantity can be split into

$$\Delta\lambda_\alpha = \Delta F_\alpha(0) - \Delta F_\alpha(\alpha) \tag{1}$$

$$= \Delta F_\alpha^{\text{elec}}(0) - \Delta F_\alpha^{\text{elec}}(\alpha) + \Delta F_\alpha^{\text{LJ}}(0) - \Delta F_\alpha^{\text{LJ}}(\alpha) + \Delta F_\alpha^{\text{int}}(0) - \Delta F_\alpha^{\text{int}}(\alpha) \tag{2}$$

In the main paper we assumed that the Lennard-Jones and the intrinsic (ideal+excess) contributions can be neglected.

$$\Delta F_\alpha^{\text{LJ}}(0) - \Delta F_\alpha^{\text{LJ}}(\alpha) = 0, \tag{3}$$

$$\Delta F_\alpha^{\text{int}}(0) - \Delta F_\alpha^{\text{int}}(\alpha) = 0. \tag{4}$$

We now verify the validity of this assumption. The two terms of equations 3 and 4 are identical for the three oxidation states. The difference in external, intrinsic and total contribution to the free energy are plotted as a function of the atomic charge used to generate the out-of equilibrium solvent density for the three oxidation states in figure 1. Since there is no electrostatics involved in the case of the neutral chlorine, the external contribution equals to the Lennard-Jones one of equation 3. The variation of $\Delta F_{\text{Cl}}^{\text{ext}}$ remains below 2.1 kJ/mol abroad the whole range of external potentials validating the hypothesis of equation 3.

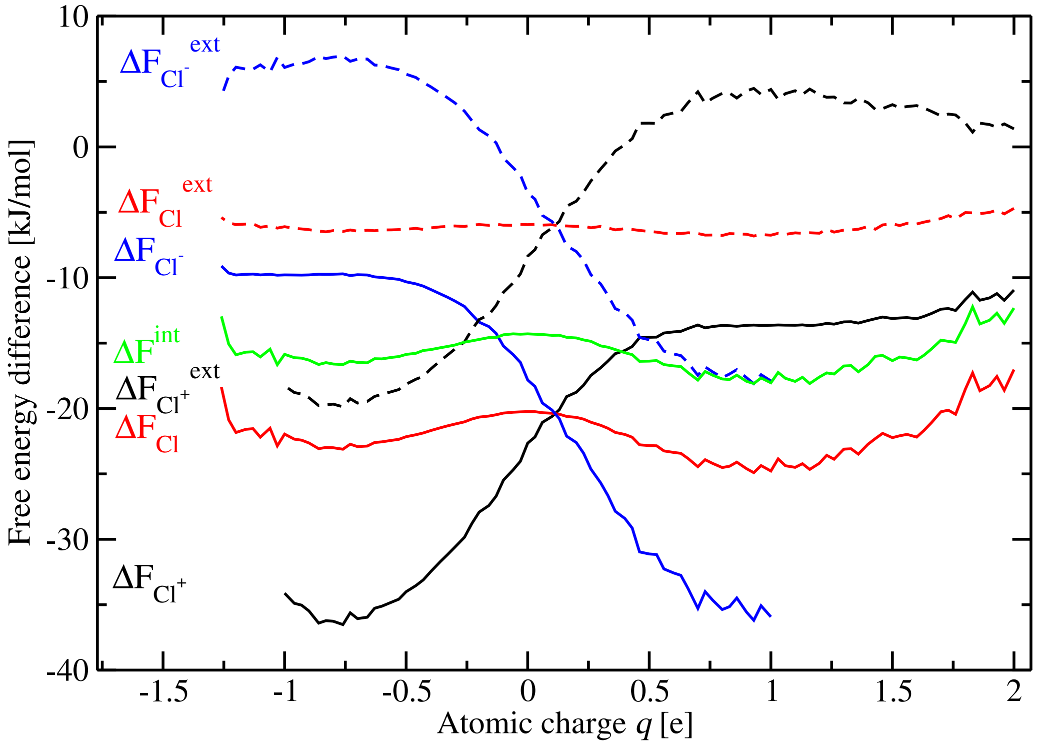


FIG. 1. Difference between functional values calculated with HNC and HNC-WDA functional

The variation of $\Delta F^{\text{int}}$ has a more pronounced amplitude than $\Delta F^{\text{LJ}}$ over the range of external potentials, but it remains below 6 kJ/mol which is considerably lower than the variation

of the external (and thus electrostatic) contribution for ions. This justifies the assumption in equation 4 and validates the approximation of equation 16 in the main paper.

Note that we also recover the qualitative arguments about the polarization made in the main article, that is $\Delta F_{\alpha}^{\mathrm{elec}}(\alpha) > 0$ and $\Delta F_{\alpha}^{\mathrm{elec}}(-\alpha) < 0$.
